# Supplementary material for: PixelRefer: A Unified Framework for Spatio-Temporal Object Referring with Arbitrary Granularity
Source: arXiv:2510.23603 source file (2025-11-01)
Supplement: Supplementary file 1 [file appendix.tex]

% \newpage
\appendix
Appendix.
